# Supplementary material for: Rethinking Prior Information Generation with CLIP for Few-Shot Segmentation
Source: arXiv:2405.08458 source file (2024-05-14)
Supplement: Supplementary file 1 [file X_suppl.tex]

% \clearpage
% \setcounter{page}{1}
% \maketitlesupplementary
\section{Ablation Study on High-order Matrix}

\begin{figure}[htbp]
	\centering
	\includegraphics[width=0.5\textwidth]{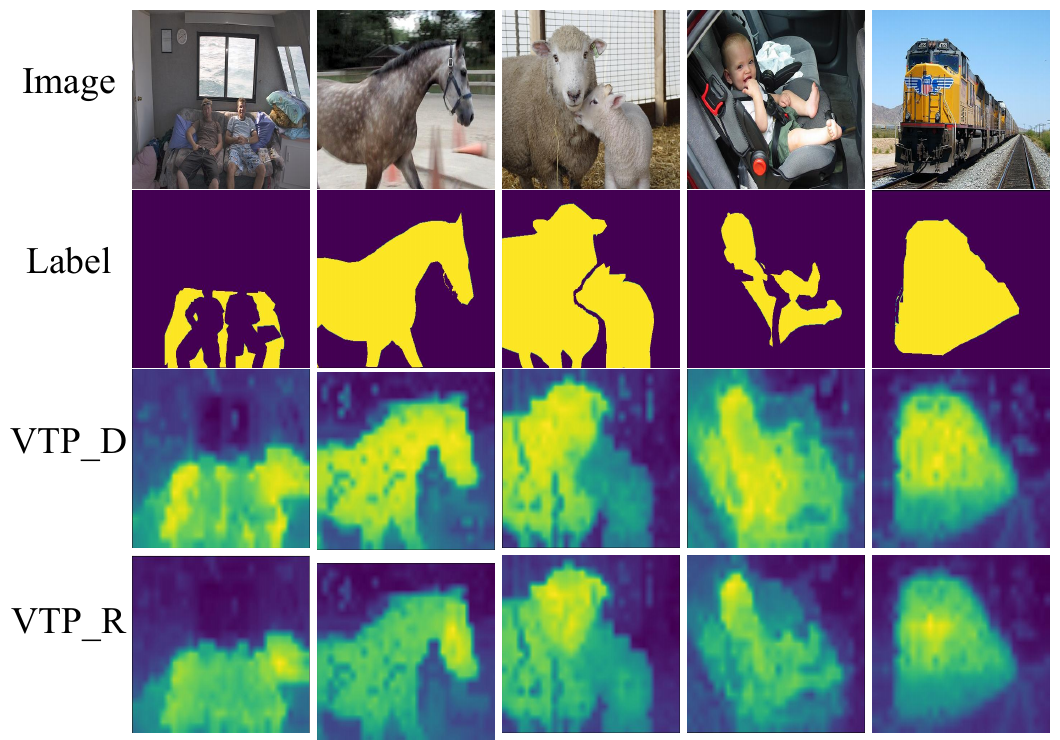}
	\caption{Qualitative results of the refinement of our designed high-order matrix. Each row from top to bottom represents the query images, query labels, refined VTP by initial matrix, and refined VTP by our proposed high-order matrix, respectively.}
	\label{fig:dd}
\end{figure}

\begin{table}[htbp]
\caption{Ablation study about our proposed high-order matrix refinement on the PASCAL-5$^{i}$, ``$D$" represents the initial matrix, $R$ represents the high-order matrix we designed.}
\centering
\begin{tabular}{cccc}
\hline
$D$ &$R$ &mIoU ($\%$) &FB-IoU ($\%$) \\
\hline
\checkmark & &75.10 &86.44\\
& \checkmark &76.40 &87.57\\
\hline
\label{tab5}
\end{tabular}
\end{table}

% \label{sec:rationale}
In order to verify the effectiveness of the higher-order matrix, we conduct ablation experiments on the effect of the higher-order matrix. As shown in Table~\ref{tab5}, when utilizing our proposed high-order matrix to refine the prior information, it gets a better performance with 76.40 mIoU $\%$ which is 1.3 $\%$ higher than utilizing the original attention matrix, and the results of the two matrix fine-tuning methods are visualized in Figure.~\ref{fig:dd}. It can be found that our proposed higher-order matrix refinement can indeed extract finer-grained prior information based on structure information and strengthen the suppression of chaotic background areas. Note that the experiments in this section follow the same setting as the experiments in the text.

\begin{table}[!t]
\caption{Ablation study about text prompts on PASCAL-5$^{i}$, $t_f$ represents the target prompt and $t_b$ represents the non-target prompt.}
\centering
\resizebox{\columnwidth}{!}{$
\begin{tabular}{ccc}
\hline
                $t_f/t_b$              &mIoU ($\%$)            &FB-IoU ($\%$) \\\hline
``a photo of \{\emph{target class}\}"  & \multirow{2}{*}{\textbf{76.40}}   & \multirow{2}{*}{\textbf{87.57}}\\
``a photo without \{\emph{target class}\}"   \\  \hline
``a photo of \{\emph{target class}\}"  & \multirow{2}{*}{71.32}    & \multirow{2}{*}{83.78}\\
``not a photo of \{\emph{target class}\}"   \\  \hline
``a clean origami of \{\emph{target class}\}"  & \multirow{2}{*}{73.97}    & \multirow{2}{*}{85.64}\\
``a clean origami different from \{\emph{target class}\}"   \\  \hline
\label{tab:text}
\end{tabular}
$}
\end{table}

\section{Ablation Study on Text Prompts} Different textual prompts directly decide the model's understanding of image visual content, which further affects the quality of the generated prior information, based on this, we conduct ablation experiments on the content of the text prompts, as shown in Table~\ref{tab:text}, the highest performance of 76.40$\%$ was achieved when using the text prompts we designed.

\section{More Visualizations}
To further demonstrate the effect of our model, we show more visualizations on the COCO-20$^{i}$~\cite{nguyen2019feature}, Figure.~\ref{fig:prior} compares more prior masks, and Figure.~\ref{fig:result_coco} provides a further visualization of the final experimental results.

\begin{figure}[!t]
	\centering
	\includegraphics[width=0.5\textwidth]{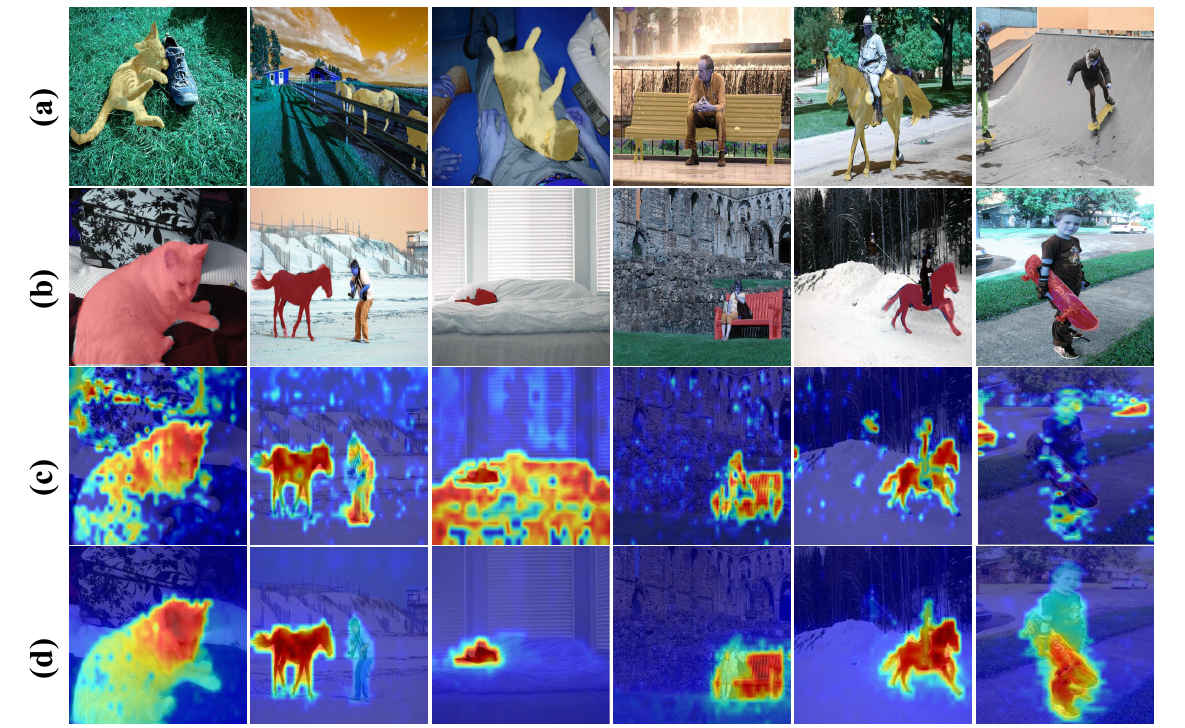}
	\caption{Comparison of more prior information from COCO-20$^{i}$~\cite{nguyen2019feature}. (a) Support images with ground-truth masks; (b) Query images with ground-truth masks; (c) Prior information from previous approaches generated based on the frozen ImageNet~\cite{deng2009imagenet} weights.}
	\label{fig:prior}
\end{figure}

\begin{figure}[htbp]
	\centering
	\includegraphics[width=0.5\textwidth]{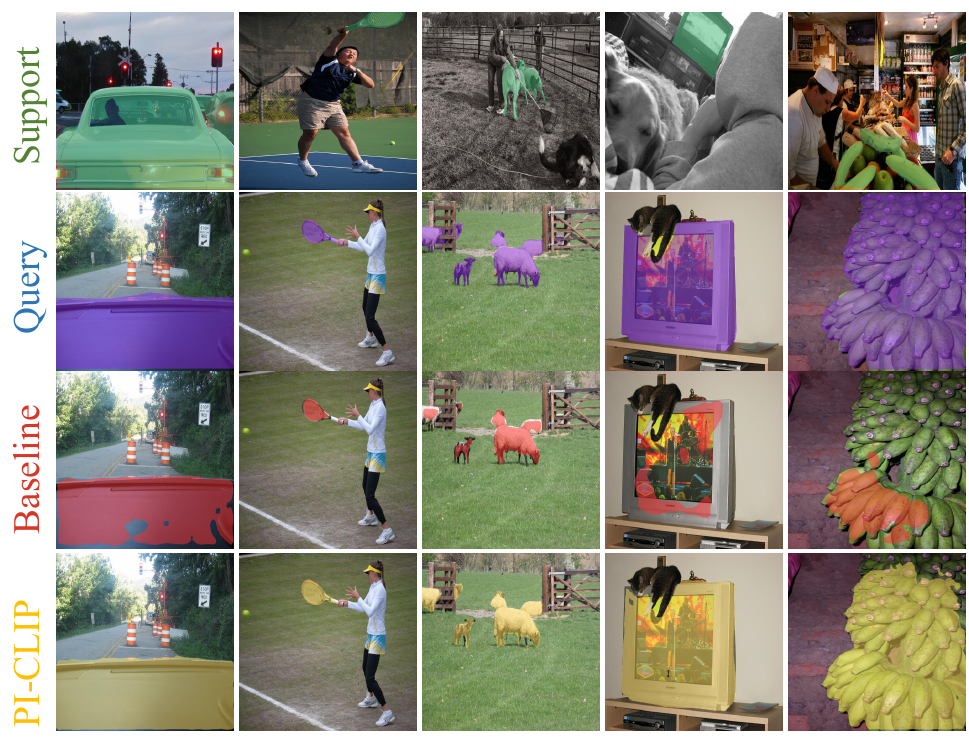}
	\caption{Qualitative results of the proposed PI-CLIP and baseline (HDMNet~\cite{peng2023hierarchical}) approach under 1-shot setting from COCO-20$^{i}$~\cite{nguyen2019feature}. Each row from top to bottom represents the support images with ground-truth  (GT) masks (green), query images with GT masks (purple), baseline results (red), and our results (yellow), respectively.}
	\label{fig:result_coco}
\end{figure}

\section{CLIP Capacity Concern: Fair Comparisons}
Not only CLIP pretraining, but also ImageNet pretraining may involve the tested novel classes. How to extract accurate features from the pretraining model and transfer them to few-shot segmentation is a more important issue than the size or capacity of the pretraining model. Besides, the CLIP model has been used in the few-shot task, \eg, CLIPSeg~\cite{luddecke2022image}, TIP-Apapter~\cite{zhang2022tip}.

\vfill\eject
